# Supplementary material for: Ensemble-Instruct: Generating Instruction-Tuning Data with a Heterogeneous Mixture of LMs
Source: arXiv:2310.13961 source file (2023-10-21)
Supplement: Supplementary file 1 [file appendix.tex]

\section{Synthetic data in the ensemble-instruct pipeline}

\section{Zero shot Performance of LMs}

\begin{table*}
%\small
\centering
\begin{tabular}{lccccc}
\hline
\textbf{Model} & \textbf{Instruction Gen.} & \textbf{Instance Gen.} & \textbf{Output Gen.} & \textbf{SuperNI} & \textbf{User-Oriented}\\
\hline
%\textsc{falcon} & Yes   & Yes  & Yes &  \\
\textsc{ul2}    & Yes   & Yes  & No & 10.4 & 7.2 \\
\textsc{gpt-neoxt-chat} & Yes & Yes & No & 6.6 & 10.2 \\
\textsc{falcon-40b} & Yes & Yes & No & 12.7 &   \\
\textsc{flan-ul2} & No   & No & Yes & 77.5 & 22.1 \\
\textsc{flan-t5-xxl} & No & No & Yes & 73.0 & 22.4 \\
\hline
\textsc{mpt-7b} & No & No & No & 16.6 & 10.6 \\
\textsc{gpt-jt-6b} & No & No & No & 10.4 & 6.2 \\
\textsc{pythia-1.4b} & No & No & No & 9.8 \\
\hline
\end{tabular}
\caption{Zero shot performance of various LMs measured in Rouge-L on SuperNI and User-Oriented test sets.}
\end{table*}

\section{Analyses}

\begin{itemize}
\item Human evaluation (2 reviewers)
\item Compare samples generated by ensemble-instruct and those by self-instruct (2 reviewers)
\item Performance comparison according to the number of outputs to ensemble (1 reviewer)
\item Performance comparison according to the number of ICL examples (1 reviewer)
\item Ensemble based on model confidence scores (1 reviewer)
\item Impact of the ensemble-instruct on downstream tasks (1 reviewer): Graphs showing the impact of sample size and quality of synthetic data
\item Explore more on vanilla model ensemble (1 reviewer)
\end{itemize}
